# Supplementary material for: A Tool for In-depth Analysis of Code Execution Reasoning of Large Language Models
Source: arXiv:2501.18482 source file (2025-01-30)
Supplement: Supplementary file 1 [file appendix.tex]

\section{Walkthrough of \name Artifact }
\subsection*{ Dependencies}
To install all the dependencies, run the following command:
\begin{verbatim}
pip install -r requirements.txt
\end{verbatim}
\name is designed to read API keys required for API-access models from local variables. Please modify and run \texttt{setup.sh {OPANAIKEY}} to automatically add the variable to your local machines.

\subsection*{Data Preparation}
Please put the dataset under \texttt{dataset} folder, and the execution reasoning results from LLMs under \texttt{Experiment\_Results/ER}.
For each problem/program in the benchmark, please create an individual folder and store its code, input, and output in \texttt{main.py}, \texttt{input.txt}, and \texttt{output.txt}, respectively. 
Concerning the code execution prediction of LLMs, store the results in a .json file named \texttt{Experiment\_Result/ER/result\_stat/\{MODEL\}\_\{DATASET\}.json}.
We provided example dataset and result in the artifact.
Please follow the format under the folder \texttt{dataset/humaneval} and the format in 
 \texttt{Experiment\_Results/result\_stat/ER/semcoder\_s\_avatar.json}

\subsection*{LLM Prompting}
Below are the commands to reproduce the code execution reasoning results of LLMs.
Users are welcomed to use their own results as long as they follow the above format in the data preparation part.

\begin{verbatim}
cd scripts
bash run_IER.sh {MODEL_ID} {CACHE_DIR} {DATASET} {PL}
\end{verbatim}

So far our framework supports the follwoing \texttt{MODEL\_ID}:
gpt-3.5-turbo, gpt-4-1106-preview, codellama/CodeLlama-13b-Instruct-hf, 
codellama/CodeLlama-13b-hf, Qwen/CodeQwen1.5-7B-Chat, Qwen/CodeQwen1.5-7B, deepseek-ai/deepseek-coder-6.7b-instruct, deepseek-ai/deepseek-coder-6.7b-base, meta-llama/Llama-2-13b-hf, ise-uiuc/Magicoder-S-DS-6.7B, mistralai/Mistral-7B-Instruct-v0.1, bigcode/starcoder, bigcode/starcoder2-15b, WizardLM/WizardCoder-15B-V1.0, gpt-4-turbo, gemini/gemini-pro, codellama/CodeLlama-7b-Instruct-hf, deepseek-ai/deepseek-llm-7b-base, gemini/gemini-1.5-pro,
semcoder/semcoder\_s.

\name supports the follwoing \texttt{DATASET}: Avatar, cruxeval, classeval, humaneval

\texttt{CACHE\_DIR} should be replaced with the path to store the downloaded pretrained huggingface model checkpoints

\subsection*{Result Analysis}
You can analyze the impact of different factors with the following commands:
\begin{verbatim}
cd analysis
\end{verbatim}
\begin{itemize}
    \item Analyze the impact of program constructs:
\begin{verbatim}
    bash analyze_construct.sh
\end{verbatim}

Output figures/stats can be found under

 \texttt{Experiment\_Results/figures/constructs}

 \item Analyze the impact of cyclomatic complexity:
\begin{verbatim}
    bash analyze_cc.sh
\end{verbatim}
Output figures/stats can be found under

\texttt{Experiment\_Results/figures/cyclomatic\_complexity}

 \item Analyze the impact of loop length:
\begin{verbatim}
    bash analyze_ll.sh
\end{verbatim}

Output figures/stats can be found under 

\texttt{Experiment\_Results/figures/loop\_length}

\item Analyze the impact of output types:

\begin{verbatim}
    bash analyze_types.sh
\end{verbatim}

Output figures/stats can be found under 

\texttt{Experiment\_Results/figures/types}

\end{itemize}
